# Supplementary material for: Shaping Next-Generation RAN Topologies to Meet Future Traffic Demands: A Peak Throughput Study
Source: arXiv:2305.03536 source file (2023-05-05)
Supplement: Supplementary file 1 [file 7_additional_material.tex]

extra page?
